# Supplementary material for: Rigidity in Mechanism Design and its Applications
Source: arXiv:2212.09847 source file (2022-12-19)
Supplement: Supplementary file 1 [file F-full-description.tex]

\section{The Distribution $\mathcal{F_S}$} \label{full_des_F}

We describe the distribution $\mathcal{F}_S$ and its domain $D_S$ from the point of view of bidder $i$, under the uniqueness of thresholds assumption (Definition~\ref{uniqueness}). 
We drop the $S$ in $\mathcal{F}_S$ and $D_S$ for simplicity of notation.

\subsection{The Support of Player $i$ }
 \begin{align*}
        D_i = & \,  \{\epsilonvalrestrictefs{i}\} \quad \text{if} \, i \in A\\
        % {\color{red!45!orange} \{\epsilonvalrestrictefs{i}\}} \\
        & \cup  \{y_{i,j}  \, | \,0 \leq  j \leq k_i+1 \} \quad \text{if} \, i \in A \\
        %  & \cup {\color{red!45!orange} \{y_{i,j}  \, | \,0 \leq  j \leq k_i+1 \}} \\
        & \cup \{ {v}_{i,j} \, | \, j \in [m] \wedge i \notin A_j\}\\
        & \cup  \{ {u'}_{i,j}, u_{i,j} \, | \, j \in [m] \wedge i \in A_j\}\\
        & \cup \{ \epsilonvaleqr{k} \, | \,  k \in A \setminus \{i\}\,  \} \\
        & \cup \{ {\epsilonvalrestrictefs{i,j}} \, | \, j \in [m] \wedge i \notin A_j\}\\
        & \cup \{ \epsilonvalrestrictefs{i,j,k} \, | \, j \in [m] \wedge k \in A_j \wedge k \neq i\}\\
        & \cup \{ \epsilonvalrestrictefs{i,j,k}' \, | \, j \in [m] \wedge k \in A_j \wedge k \neq i\}
    \end{align*}

\subsection{The Marginal Distribution of Player $i$} \label{marginal}
    \begin{align*}
        % & \Pr\nolimits_{\mathcal{F}_i}(v_i = \epsilonvalrestrictefs{i}) = \epsilonprob{} &\\
        & \Pr\nolimits_{\mathcal{F}_i}(v_i = \epsilonvalrestrictefs{i}) = \begin{cases*}
        \epsilonprob{} & \text{if $ i \in A$}\\
        0 & \text{if $i \notin A$}
        \end{cases*}& \\
        & \Pr\nolimits_{\mathcal{F}_i}(v_i = v_{i,j}) =  \begin{cases*}
         \frac{1-\delta}{\sizeActive}\cdot q_{i,j} + \basevectorprob{j} + \epsilonprob{} \cdot 2(|A_j|-1) & \text{if $ i \in A_j$}\\
        \basevectorprob{j} +\epsilonprob{}\cdot 2|A_j| & \text{if $i \notin A_j$}
        \end{cases*} & \forall j \in [m]\\ 
        % & \Pr\nolimits_{\mathcal{F}_i}(v_i = y_{i,j}) =  \frac{1-\epsilonprob{}}{n}\cdot q_i^j  & \forall j \in \{0, k_i + 1\} \\
        & \Pr\nolimits_{\mathcal{F}_i}(v_i = y_{i,j}) =  \begin{cases*}
         \frac{1-\epsilonprob{}}{\sizeActive}\cdot q_{i,j} & \text{if $ i \in A$}\\
        0 & \text{if $i \notin A$}
        \end{cases*} & \forall j \in \{0, k_i + 1\} \\ 
        % & \Pr\nolimits_{\mathcal{F}_i}(v_i = v_{i,t}) =  \basevectorprob{t} + \epsilonprob{} \cdot(|A_t|) & \forall t \in [m] \; \forall i \notin A_t\\ 
        % & \Pr\nolimits_{\mathcal{F}_i}(v_i = {u'}_{i,j}) =  \epsilonprob{} & \forall j \in [m] \wedge i \in A_j\\
        & \Pr\nolimits_{\mathcal{F}_i}(v_i = {u'}_{i,j}) = \epsilonprob{}  & \forall j \in A_i  \\
        & \Pr\nolimits_{\mathcal{F}_i}(v_i = {u}_{i,j}) =  \epsilonprob{}  & \forall j \in A_i  \\
        & \Pr\nolimits_{\mathcal{F}_i}(v_i = \epsilonvaleqr{k}) = \frac{1-\delta}{\sizeActive} & \forall k \in A\setminus \{i\}\\
        & \Pr\nolimits_{\mathcal{F}_i}(v_i = \epsilonvalrestrictefs{i,t}) = \epsilonprob{} & \forall t \in [m] \; \forall i \notin A_t\\
        & \Pr\nolimits_{\mathcal{F}_i}(v_i = \epsilonvalrestrictefs{i,j,k}) = \epsilonprob{} & \forall  j \in [m] \; \forall k \in A_j \setminus \{i \} \\  
        & \Pr\nolimits_{\mathcal{F}_i}(v_i = \epsilonvalrestrictefs{i,j,k}') = \epsilonprob{} & \forall  j \in [m] \; \forall k \in A_j \setminus \{i \} \\   
    \end{align*}

% Observe that the only values of player $i$ that can fit to more than one row are of the form $u_{i,j}$ and then these are the three options; The first is that $u_{i,j} = y_{i,k}$ for some value of $k \in [m]$ such that $ i \in A_k$ and $k \neq j$. The second option is $u_{i,j} = v_{i,t}$ for some value of $t \in [m]$ such that $ i \notin A_t$. The third and last option is that $u_{i,j} = u_{i,r}$  for some value of $r \in [m]$ such that $ r \neq j$.

\subsection{The Conditional Probability of $v_{-i}$ Given $v_i$}
        \begin{align*}
        & \Pr\nolimits_{F}(v_{-i} = (v_{j})_{-i} \, |\,  v_i = v_{i,j}) =  & \\ 
        & \qquad \begin{cases*}
         \frac{\basevectorprob{j}}{ \Pr\nolimits_{\mathcal{F}_i}(v_i = v_{i,j})} \underbrace{=}_{\text{denote by}} \basevectorprob{i,j} & \text{if $ i \in A_j$}\\
        \frac{\basevectorprob{j}}{ \Pr\nolimits_{\mathcal{F}_i}(v_i = v_{i,j})} & \text{if $i \notin A$}
        \end{cases*} & \forall j \in [m] \\ 
        & \Pr\nolimits_{F}(v_k,v_{-i-k}) = ({u'}_{j,k},({v}_{j})_{-i-k} ) \, |\,  v_i = v_{i,j}) =  \Pr\nolimits_{F}(v_k,v_{-i-k}) = ({u}_{j,k},({v}_{j})_{-i-k} ) \, |\,  v_i = v_{i,j}) = &\\ & \qquad \begin{cases*}
         \frac{ \epsilonprob{}}{  \Pr\nolimits_{\mathcal{F}_i}(v_i = v_{i,j})} \underbrace{=}_{\text{denote by}} \frac{\epsilonprob{i,j}}{2(|A_j| -1)} & \text{if $ i \in A_j$}\\
        \frac{\epsilonprob{}}{ \Pr\nolimits_{\mathcal{F}_i}(v_i = v_{i,j})} & \text{if $i \notin A_j$}
        \end{cases*} & \forall j \in [m] \; \forall k \in A_j \setminus \{i\} \\ 
        & \Pr\nolimits_{F}(v_{-i} = \epsilonvaleqr{i} \dots \epsilonvaleqr{i} \, |\,  v_i = v_{i,j}) = &\\
        & \qquad \begin{cases*}
        1-\basevectorprob{i,j} -\epsilonprob{i,j} & \text{if $ i \in A$}\\
        0 & \text{if $i \notin A$}
        \end{cases*} &  \forall j \in [m] \; \forall i \in A_j \\
         & \Pr\nolimits_{F}((v_k,v_{-i-k}) = ({u'}_{j,k},({v}_{j})_{-i-k})| v_i= \epsilonvalrestrictefs{i,j,k}) = 1 &  \forall j \in [m] \; \forall k \in A_j \setminus\{i\}\\  
        & \Pr\nolimits_{F}((v_k,v_{-i-k}) = ({u}_{j,k},({v}_{j})_{-i-k})| v_i= \epsilonvalrestrictefs{i,j,k}') = 1 &  \forall j \in [m] \; \forall k \in A_j \setminus\{i\}\\  
        & \Pr\nolimits_{F}(v_{-i} = \epsilonvaleqr{i} \dots \epsilonvaleqr{i} \, |\,  v_i = y_{i,j})  = & \\
        & \qquad \begin{cases*}
        1 & \text{if $ i \in A$}\\
        0 & \text{if $i \notin A$}
        \end{cases*} &  \forall j \in \{0, k_i+1\}\\
        & \Pr\nolimits_{F}(v_{-i} = (v_j)_{-i} \, |\,  v_i = {u'}_{i,j}) =  1  &   \forall j \in  A_i\\ 
        & \Pr\nolimits_{F}(v_{-i} = (v_j)_{-i} \, |\,  v_i = {u}_{i,j}) = 
        1  &   \forall j \in  A_i\\ 
        & \Pr\nolimits_{F}(v_{-i} = (v_{t})_{-i} \, |\,  v_i = \epsilonvalrestrictefs{i,t}) = 1 &  \forall t \in [m] \wedge i \notin A_t \\
        & \Pr\nolimits_{F}(v_r,v_{-i-r}) = ({y}_{r,j},\epsilonvaleqr{r} \dots \epsilonprob{r}) \, |\,  v_i = \epsilonprob{r}) =  q_{r,j} &  \forall\: (r \in A \setminus \{i\}) \; \forall \: (0 \leq j \leq k_r+1)\\
        \end{align*}

% \subsection{Conditional Probability Matrix of a non-active Player}
% \begin{figure}[H]
%     \centering
% \begin{align*}
%     % & CP_i(\mathcal{F}_S)= \\
%     & \begin{pNiceMatrix}[first-row,first-col] 
%     &  \dots & {\color{red!45!orange}(v_t)_{-i}} & \dots & {\color{green!70!black}({u'}_{l,j}, (v_j)_{-i-l})} & \dots & {\color{violet}y_{r,0}} & \dots & {\color{violet} y_{r,{k_r +1}}}\\
%     \vdots & \dots  & \dots  & \dots  & \dots  & \dots  & \dots  & \dots  & \dots \\
%     {\color{red!45!orange} {v}_{i,t} }&\dots & \frac{\basevectorprob{j}}{\basevectorprob{j} +\epsilonprob{} \cdot |A_j|} & \dots & \frac{\epsilonprob{}}{\basevectorprob{j} +\epsilonprob{ }\cdot |A_j|} &  \dots & 0 & \dots  &0 \\
%      \vdots &  \dots & \dots & \dots & \dots & \dots & \dots & \dots &\dots  \\
%     {\color{red!45!orange} \epsilonvalrestrictefs{i,t}} &\dots & 1 & \dots & 0 & \dots & 0 & \dots  & 0 \\
%     \vdots &  \dots & \dots & \dots & \dots & \dots & \dots & \dots &\dots  \\    
%     {\color{green!70!black}{\epsilonvalrestrictefs{i,t,l}}} & \dots & 0 & \dots & 1 & \dots & 0 & \dots & 0  \\ 
%     \vdots &  \dots & \dots & \dots & \dots & \dots & \dots & \dots &\dots  \\    
%     {\color{violet}\epsilonvaleqr{r}} & \dots & 0 & \dots & 0 & \dots & q_{r,0} &\dots & q_{r,{k_r+1}} \\
%     \vdots &  \dots & \dots & \dots & \dots & \dots & \dots & \dots &\dots  \\    
%     \end{pNiceMatrix}
% \end{align*}
%     \caption{$ CP_i(\mathcal{F})$ : The conditional probability matrix of a non-active player $i \in A$}
%     \label{CPM_not_active}
% \end{figure}
