# Supplementary material for: Rigidity in Mechanism Design and its Applications
Source: arXiv:2212.09847 source file (2022-12-19)
Supplement: Supplementary file 2 [file proof-without-assumption.tex]

\section{Removing the Uniqueness of Thresholds Assumption}\label{no_asm}

Removing the uniqueness of thresholds assumption (Assumption~\ref{uniq_assumption}) requires some modifications, but the proof largely remains the same. In particular, the construction of the subdistributions $P, E, O$ and $R$ is the same. However, their union $\mathcal{F}_S$ can have a different marginal and conditional probabilities than before (see Section~\ref{no_asm_f_s}), since now the same value of a threshold $u_{i,j}$ for player $i$ can repeat in different subsets that he is active in (i.e., $u_{i,j} = u_{i,k}$ for different $j,k \in \Asetforplayer{i}$) and this value $u_{i,j}$ can also be equal to one of player's $i$ values in the base vectors (i.e., $u_{i,j} = v_{i,k}$ for different $j,k$ $j\in \Asetforplayer{i}$ ).
Next, we define some variables that describe the colliding values.
The required changes in the analysis part of the proof (Section~\ref{analysis_of_revenue}) are described in Section~\ref{no_asm_revenue}.

%We define some variables to describe the colliding values. 
\begin{itemize}
    \item For every player $i$ and every subset $j$, let $\cntvaluedcolliding{i,j} = |\{u_{i,k} | u_{i,k} = v_{i,j}, k \in \Asetforplayer{i} \}|$.
    \item For every player $i$ and every $j\in \Asetforplayer{i}$, let $\cntthresholdcolliding{i,j} = |\{u_{i,k} | u_{i,k} = u_{i,j}, k \in \Asetforplayer{i} \}|$.
    \item For every player $i$ and every $j\in \Asetforplayer{i}$, let $\indthresholdcolliding{i,j} = \begin{cases*}
        1 & \text{if $ \exists\,  k \in [m]$ s.t. $ u_{i,j} = v_{i,k}$};\\
        0 & \text{otherwise}.
    \end{cases*}$
\end{itemize}

\subsection{Description of $\mathcal{F}_S$} \label{no_asm_f_s}

\note{Doesn't take into account the instances in R!}
These are the changes to the marginal distribution of player $i$, $\mathcal{F}_i$:
    \begin{align*}
        & \Pr\nolimits_{\mathcal{F}_i}(v_i = v_{i,j}) =  \begin{cases*}
         \frac{1-\delta}{\sizeActive}\cdot q_{i,j} + \basevectorprob{j} + \epsilonprob{} 2\cdot(|A_j|-1 + w_{i,j}) & \text{if $ i \in A_j$};\\
        \basevectorprob{j} +\epsilonprob{}\cdot 2(|A_j| + w_{i,j}) & \text{if $i \notin A_j$}.
        \end{cases*} & \forall j \in [m]\\ 
        & \Pr\nolimits_{\mathcal{F}_i}(v_i = {u}_{i,j}) =  \begin{cases*}
         \epsilonprob{}\cdot c_{i,j} & \text{if $ s_{i,j} =0 $};\\
        \Pr\nolimits_{\mathcal{F}_i}(v_i = v_{i,k}) & \text{o.w $s_{i,j} =1$ and then $\exists k \in [m]$ s.t. $ v_{i,k} = u_{i,j}$.}
        \end{cases*} & \forall j \in [m]\\ 
    \end{align*}
These are the changes to the conditional probability of the values of the other player, given that player $i$'s value is $v_i$:
 \begin{align*}
         \Pr\nolimits_{\mathcal F_S}(v_k,v_{-i-k}) = ({u}_{j,k},({v}_{j})_{-i-k} ) \, |\,  v_i = v_{i,j}) &=\begin{cases*}
         \frac{ \epsilonprob{}}{  \Pr\nolimits_{\mathcal{F}_i}(v_i = v_{i,j})} \underbrace{=}_{\text{denote by}} \frac{\epsilonprob{i,j}}{(2|A_j| -2 +w_{i,j})} & \text{if $ i \in A_j$};\\
        \frac{\epsilonprob{}}{ \Pr\nolimits_{\mathcal{F}_i}(v_i = v_{i,j})} & \text{if $i \notin A_j$.}
        \end{cases*} & \ \ \ (\forall j \in [m] \; \forall k \in A_j \setminus \{i\}) \\ 
        \Pr\nolimits_{\mathcal F_S}(v_k,v_{-i-k}) = ({u'}_{j,k},({v}_{j})_{-i-k} ) \, |\,  v_i = v_{i,j}) &=\begin{cases*}
         \frac{ \epsilonprob{}}{  \Pr\nolimits_{\mathcal{F}_i}(v_i = v_{i,j})} \underbrace{=}_{\text{denote by}} \frac{\epsilonprob{i,j}}{(2|A_j| -2 +w_{i,j})} & \text{if $ i \in A_j$};\\
        \frac{\epsilonprob{}}{ \Pr\nolimits_{\mathcal{F}_i}(v_i = v_{i,j})} & \text{if $i \notin A_j$.}
        \end{cases*} & \ \ \ (\forall j \in [m] \; \forall k \in A_j \setminus \{i\}) \\ 
         \Pr\nolimits_{\mathcal F_S}(v_{-i} = (v_k)_{-i} \, |\,  v_i = v_{i,j}) &= 
         \begin{cases*}
        \frac{\epsilonprob{}}{\Pr\nolimits_{\mathcal{F}_i}(v_i = v_{i,j})} & \text{if $ v_{i,j} = u_{i,k}$;}\\
        0 & \text{otherwise. }
        \end{cases*}   (\forall j \in [m] \; \forall k \in A_i) \\
         \Pr\nolimits_{\mathcal F_S}(v_{-i} = (v_k)_{-i} \, |\,  v_i = u_{i,j}) &= 
      \begin{cases*}
        \frac{\epsilonprob{}}{\epsilonprob{}\cdot c_{i,j}} & \text{if $ u_{i,j} = u_{i,k}$};\\
        0 & \text{otherwise.}
        \end{cases*}  \ \ \  (\forall j \in [m] \; \forall k \in A_i) \\
        \end{align*}

\subsection{Extracting Revenue in the Distribution $\mathcal{F}_S$} \label{no_asm_revenue}

The general form of the proof remains as all the statements of the propositions, claims and lemmas are the same. However, some proofs need to be slightly modified.

The issue is that the row vector in the conditional probability matrix of player $i$ $[CP_i(\mathcal{F})]$ that corresponds to the value $u_{i,j}$ might be different. With the assumption, this vector had 0 entries everywhere except for the column that corresponds to $v_{-i} = \vec{v_j}_{-i}$. Now, this vector can have additional non-zero entries, as this value might collide with other thresholds of player $i$ or one of his values in the base vectors. 

The proof of Proposition~\ref{lower_bound_on_revenue} is almost the same.
The described interim IR mechanism that is constructed does not assume the uniqueness of thresholds assumption and thus the only difference is the analysis of its fees.
This analysis (actually only Item~\ref{u_lb}) requires a small modification that takes into account the slightly changed conditional probability (Section~\ref{no_asm_f_s}). 

% \sdcomment{last sentence is not grammatically correct and I don't understand what you mean}\ascomment{Is it better now? or do you think I should just prove it again here}

We now discuss the proof of Proposition~\ref{upper_bound_on_revenue}. The proof is the same except for the proofs of two lemmas; Lemma~\ref{lemma:efs_depends_on_S} and Lemma~\ref{lemma:fees_bound_per_val} that we will prove now without using the uniqueness of thresholds assumption. 

For this analysis we might need even smaller values of $\epsilonprob{}$ that is defined in Section \ref{O} \footnote{Recall that this variable is arbitrarily small and so further decreasing have no significant effect.} and thus we require that the value of $\epsilonprob{}$ will also satisfy:

\begin{equation} \label{nasm_cond_epsilon}
    \epsilonprob{} \leq \frac{\epsilonvallowest \cdot \min\limits_{j \in [m]} \basevectorprob{j}^2 \cdot(1-\basevectorprob{})}{\max\limits_{i \in [n]}|D_{-i}|\cdot\max\limits_{j \in [m], i \in A_j}\{u_{i,j}\} }
\end{equation}

% \begin{lemma}
% For every $ j\in [m]$, $i \in \Asetforsubset{j}$, $(v_j)_{-i}$, if the mechanism $\expostmechanism$ does not allocate the item to bidder $i$ in the instance $(u_{i,j}, (v_j)_{-i})$, then $c_i((v_j)_{-i}) \leq 0$. 
% \end{lemma}

%(in a later section)

% \begin{lemma:efs_depends_on_S}
% For every $ j\in [m]$, $i \in \Asetforsubset{j}$, $(v_j)_{-i}$, if the mechanism $\expostmechanism$ does not allocate the item to bidder $i$ in the instance $(u_{i,j}, (v_j)_{-i})$, then $c_i((v_j)_{-i}) \leq 0$. 
% \end{lemma:efs_depends_on_S}

\begin{proof}[Proof of Lemma~\ref{lemma:efs_depends_on_S} without the uniqueness of thresholds assumption]

Now we cannot assume that the row vector in the conditional probability matrix of player $i$ $[CP_i(\mathcal{F})]$ that corresponds to $u_{i,j}$ has $0$ entries everywhere except for the column that corresponds to $v_{-i} = \vec{v_j}_{-i}$ and so we use the variable $u'_{i,j}$ (defined in Section~\ref{O}) instead.

Most of the proof is based on the same arguments that the previous proof uses, only this time we apply them to $u'_{i,j}$ instead. The difference is that we need to connect between the allocation of $\expostmechanism$ in the instance $(u_{i,j}, (v_j)_{-i})$ and the profit of player $i$ when his value is $u'_{i,j}$.

For every player $i$ and every subset $S_j$ that player $i$ is active in we defined $u'_{i,j}$ that satisfies $u'_{i,j} \leq u_{i,j}$ and that his corresponding row 
vector in the conditional probability matrix of player $i$ $[CP_i(\mathcal{F})]$ has $0$ entries everywhere except for the column that corresponds to $v_{-i} = \vec{v_j}_{-i}$. Therefore:

\begin{subequations} 
\begin{equation}\label{u_value_prof_nasm}
    \pi_i^{\expostmechanism(\mathcal{F})}({{u'}_{i,j}}) = \pi_i^{\expostmechanism(\mathcal{F})}({{u}'_{i,j}}, \vec{v_j}_{-i})
\end{equation}
\begin{equation}\label{u_value_fee_nasm}
    {[CP_i(\mathcal{F})]_{(u'_{i,j})}\cdot \Vec{c_i}^{\top}} = c_i(\vec{v_j}_{-i})
\end{equation}
\end{subequations}

Assume that $\expostmechanism$ does not allocate the item to player $i\in \Asetforsubset{j}$ in the instance $(u_{i,j}, (v_j)_{-i})$. Then, since $\expostmechanism$ is a dominant strategy incentive compatible mechanism he also does not allocate the item to player $i$ in the instance $(u'_{i,j}, (v_j)_{-i})$ since $u'_{i,j} \leq u_{i,j}$ \footnote{Recall that we only have one item and thus the allocation function of a dominant strategy incentive compatible mechanism must be monotone.}.

\begin{equation} \label{profit_0_u_nasm}
    \pi_i^{\expostmechanism(\mathcal{F})}({{u'}_{i,j}}, \vec{v_j}_{-i}) = 0
\end{equation}

By Equation~\ref{characterizarion_condition}  we have:
\begin{equation} \label{fees_by_profit_u_nasm}
{[CP_i(\mathcal{F})]_{(u'_{i,j})}\cdot \Vec{c_i}^{\top}} \leq \pi_i^{\expostmechanism(\mathcal{F})}({{u'}_{i,j}})
\end{equation}

Combining Equation~\ref{u_value_prof_nasm}, Equation~\ref{u_value_fee_nasm},  Equation~\ref{profit_0_u_nasm}, and Equation~\ref{fees_by_profit_u_nasm}, we get:

$$
c_i(\vec{v_j}_{-i}) \leq \pi_i^{\expostmechanism(\mathcal{F})}({{u'}_{i,j}}, \vec{v_j}_{-i}) = 0
$$
\end{proof}

% \begin{lemma:fees_bound_per_val}
% Fix a player $i\in [n]$ and a value in his support $w_i \in D_i$. It holds that:
% \begin{align*}
% \Pr\nolimits_{\mathcal{F}_i}(v_i = w_i)\cdot {[CP_i(\mathcal{F})]_{(w_i)}\cdot \Vec{c_i}^{\top}} \leq
% \begin{cases}
% \epsilonvallowest & \text{if $w_i \neq v_{i,j}$ for every $j \in A_i$};\\
% \epsilonvallowest + \feesbasevec{i,j}  & \text{if $w_i = v_{i,j}$ for some $j \in A_i$.}
% \end{cases}
% \end{align*}
% \end{lemma:fees_bound_per_val}

To prove Lemma~\ref{lemma:fees_bound_per_val}, we use the following observation. 

\begin{observation}\label{ths_fees}
Assume that player $i$ has value $v_i = v_{i,j}$ for some subset $S_j$. Then, every $v_{-i} = \vec{v_k}_{-i}$ for subset $S_k$ that is different from $S_j$ (i.e., $j \neq k$), satisfies:
% and has non-zero probability when $v_i = w_i$, (i.e., $\Pr\nolimits_{F}(v_{-i} = w_{-i} \, |\,  v_i = w_i) > 0 $)
$$
{[CP_i(\mathcal{F})]}_{(v_{i,j}, \vec{v_k}_{-i})} \cdot c_i(\vec{v_k}_{-i}) \leq \frac{\epsilonvallowest}{|D_i|}
$$
\end{observation}

\begin{proof}[Proof of Observation~\ref{ths_fees}]
Let $v_{-i} = \vec{v_k}_{-i}$ be as in the observation's statement. Then,  from Lemma~\ref{lemma:fees_base_vector} we have (\eqref{bound_ci}) and from Equation~\eqref{nasm_cond_epsilon} we have (\eqref{bound_ex_ci}):
    \begin{subequations}
    \begin{equation} \label{bound_ci}
        c_i(\vec{v_k}_{-i}) \leq \frac{\feesbasevec{i,j}}{\basevectorprob{j}}
    \end{equation}
    \begin{equation} \label{bound_ex_ci}
        \frac{\epsilonprob{}}{\Pr\nolimits_{\mathcal{F}_i}(v_i = v_{i,j})} \cdot \max\limits_{j \in A_i}\feesbasevec{i,j} \leq \frac{\epsilonvallowest \cdot \min\limits_{j \in [m]}\basevectorprob{j}}{|D_{-i}|}
    \end{equation}
    \end{subequations}
    Combining it together we get:
    \begin{align*}
        {[CP_i(\mathcal{F})]}_{(v_{i,j}, \vec{v_k}_{-i})} \cdot c_i(\vec{v_k}_{-i}) \leq  \frac{\epsilonprob{}}{\Pr\nolimits_{\mathcal{F}_i}(v_i = v_{i,j})} \cdot c_i(\vec{v_k}_{-i}) \leq \frac{\epsilonvallowest}{|D_i|}
    \end{align*}
\end{proof} 

\begin{proof}[Proof of Lemma~\ref{lemma:fees_bound_per_val} without the uniqueness of thresholds assumption]
We go over all the values $w_i \in D_i$ of player $i$ and this time we take into account the possible collisions in the values. 
 
% Observation~\ref{bound_on_every_v_-i} still hold and we prove another useful observation for the analysis of this lemma. 

\begin{itemize}
    \item  \emph{$w_i = v_{i,t}$  for some subset $S_t$ that player $i$ is not active in}. This value satisfies the first condition in the statement of the lemma. Recall that $w_{i,t}$ is the number of threshold values for different subsets $S_j$ that equal to the value $v_{i,t}$. 
    Now, by Observation~\ref{bound_on_every_v_-i}, Observation~\ref{ths_fees}, and Observation~\ref{efs_upper_bound} we get:
    \begin{align*}
        \Pr\nolimits_{\mathcal{F}_i}(v_i = v_{i,t})\cdot {[CP_i(\mathcal{F})]_{(v_{i,t})}\cdot \Vec{c_i}^{\top}} \leq \epsilonvallowest
        % \leq \frac{\basevectorprob{t}}{\Pr\nolimits_{\mathcal{F}_i}(v_i = v_{i,t})}\cdot \epsilonvallowest + \frac{w_{i,t} \cdot \epsilonprob{}}{\Pr\nolimits_{\mathcal{F}_i}(v_i = v_{i,t})}\cdot \max\limits_{j \in A_i} \feesbasevec{i,j} \underbrace{\leq}_{Equation~\eqref{nasm_cond_epsilon}} \epsilonvallowest. 
    \end{align*}
    \item \emph{$w_i = y_{i,0}$ or $w_i = y_{i,k+1}$}. If $w_i \leq \epsilonvallowest$, then due to Observation~\ref{efs_bounded_by_value} we get the required bound. Otherwise, by Observation~\ref{bound_on_every_v_-i} (as $w_i > \epsilonvallowest$) and Observation~\ref{efs_upper_bound} we get:
    $$
    \Pr\nolimits_{\mathcal{F}_i}(v_i = v_{i,t})\cdot {[CP_i(\mathcal{F})]_{(v_{i,t})}\cdot \Vec{c_i}}  \leq \Pr\nolimits_{\mathcal{F}_i}(v_i = v_{i,t}) \cdot \epsilonvallowest \leq \epsilonvallowest.
    $$
    \item \emph{$w_i \neq v_{i,k}$ for every subset $S_k$ and $w_i \neq y_{i,0}, y_{i,k_i+1}$}. Then, $\Pr\nolimits_{\mathcal{F}_i}(v_i = w_i) \leq m \cdot\epsilonprob{}$ and since $m \cdot \epsilonprob{} \cdot \max\limits_{j \in [m]} \{ \max\limits_{i \in \Asetforsubset{j}} \{u_{i,j}\} \} \leq \epsilonvallowest$ (by the condition in Equation~\ref{smaller_than_lowest}) we get:
    $$
    \Pr\nolimits_{\mathcal{F}_i}(v_i = w_i)\cdot {[CP_i(\mathcal{F})]_{(w_i)}\cdot \Vec{c_i}^{\top}} \underbrace{\leq}_{Observation~\ref{efs_upper_bound}}\Pr\nolimits_{\mathcal{F}_i}(v_i = w_i)\cdot w_i \leq \epsilonvallowest.
    $$
    \item \emph{$w_i = v_{i,j}$ for some subset $S_j$.}
    By Observation~\ref{bound_on_every_v_-i}, Observation~\ref{ths_fees}, and Observation~\ref{efs_upper_bound} we get:
    \begin{align*}
    \Pr\nolimits_{\mathcal{F}_i}(v_i = v_{i,j})\cdot {[CP_i(\mathcal{F})]_{(v_{i,j})}\cdot \Vec{c_i}^{\top}} & \leq  \Pr\nolimits_{\mathcal{F}_i}(v_i = v_{i,j})\cdot 
    (\basevectorprob{i,j}\cdot [\vec{c_i}]_{({v_j}_{-i})} + \epsilonvallowest) \\
    & = \basevectorprob{j} \cdot [\vec{c_i}]_{({v_j}_{-i})} + \epsilonvallowest
    \underbrace{\leq}_{Lemma~\ref{lemma:fees_base_vector}} \epsilonvallowest + \feesbasevec{i,j} 
    \end{align*}
\end{itemize}
\end{proof}
